# Supplementary material for: Designing Virtual Reality Games for Grief: A Workshop Approach with Mental Health Professionals
Source: arXiv:2512.17025 source file (2025-12-18)
Supplement: Supplementary file 1 [file appendix.tex]

\appendix

\input{figures and tables/tab-questions}
\input{figures and tables/tab-survey}
\input{figures and tables/tab-demo-info}
